# Supplementary material for: Nonreciprocal transport based on cavity Floquet modes in optomechanics
Source: arXiv:1912.10541 ancillary file (2019-12-22)
Supplement: Supplementary file 1 [file SI.pdf]

# SI: Nonreciprocal transport based on cavity Floquet modes in optomechanics

Laure Mercier de Lépinay, Caspar F. Ockeloen-Korppi, Daniel Malz, and Mika A. Sillanpää

## I. DEVICE INTRINSIC PARAMETERS

|                                       |                                  |          |
|---------------------------------------|----------------------------------|----------|
| Primary cavity frequency              | $\omega_c/2\pi$                  | 4.98 GHz |
| Primary cavity external decay rate    | $\kappa_e/2\pi$                  | 1.31 MHz |
| Primary cavity internal decay rate    | $\kappa_i/2\pi$                  | 190 kHz  |
| Primary cavity total linewidth        | $(\kappa_e + \kappa_i)/2\pi$     | 1.50 MHz |
| Auxiliary cavity frequency            | $\omega_c^a/2\pi$                | 6.62 GHz |
| Auxiliary cavity external decay rate  | $\kappa_e^a/2\pi$                | 903 kHz  |
| Auxiliary cavity internal decay rate  | $\kappa_i^a/2\pi$                | 575 kHz  |
| Auxiliary cavity total linewidth      | $(\kappa_e^a + \kappa_i^a)/2\pi$ | 1.48 MHz |
| Mechanical mode 1 frequency           | $\Omega_1/2\pi$                  | 6.69 MHz |
| Mechanical mode 1 intrinsic linewidth | $\gamma_1^0/2\pi$                | 55 Hz    |
| Mechanical mode 2 frequency           | $\Omega_2/2\pi$                  | 9.03 MHz |
| Mechanical mode 2 intrinsic linewidth | $\gamma_2^0/2\pi$                | 110 Hz   |
| Optomechanical coupling ratios        | $g_2/g_1$                        | 0.709    |
|                                       | $g_1^a/g_1$                      | 0.632    |
|                                       | $g_2^a/g_1$                      | 0.431    |

## II. BASIC THEORY

The optomechanical Hamiltonian in the laboratory frame is

$$H/\hbar = \omega_c a^\dagger a + \sum_j \Omega_j b_j^\dagger b_j - \sum_j g_j a^\dagger a (b_j^\dagger + b_j) \quad (\text{S1})$$

The system is pumped at  $\{\omega_c - (\Omega_i + \delta_i) - \Delta\}_{i=1,2}$ , that is, close to red sidebands, and at  $\{\omega_c \pm (\Omega_i + \delta_i) + \Delta\}$  with the + sign corresponding to the amplifier configuration (then these frequencies are close to blue sidebands) and the − sign corresponding to the isolator (red sidebands). The intracavity field is developed into

$$a(t) = e^{-i\omega_c t} \left[ \sum_j \left( \alpha_{j-} e^{i(\Omega_j + \delta_j - \Delta)t} + \alpha_{j+} e^{\pm i(\Omega_j + \delta_j \pm \Delta)t} \right) + \tilde{a}(t) \right] = e^{-i\omega_c t} \left[ \sum_j \alpha_j(t) + \tilde{a}(t) \right] \quad (\text{S2})$$

where  $\alpha_{j-}$  represents the classical intracavity field amplitude at the frequency of the pumps detuned by  $-\Delta$ , which are close to red sidebands in both modes of operation,  $\alpha_{j+}$  is the field amplitude of the pumps detuned by  $+\Delta$ , which are close to red sidebands in the case of the isolator and to blue sidebands in the case of the amplifier, and  $\tilde{a}(t)$  represents any other components of the field, assumed to be very small compared to the strong pumped fields. This allows to carry out the usual linearization of the optomechanical Hamiltonian, which, after moving into the frame rotating with  $H_0/\hbar = \omega_c a^\dagger a + \sum_j (\Omega_j + \delta_j) b_j^\dagger b_j$  yields:

$$H_{\text{rot}}/\hbar = -\delta_i b_i^\dagger b_i - \sum_j g_j \left[ \alpha_j^*(t) \tilde{a}(t) \left( b_i^\dagger e^{i(\Omega_i + \delta_i)t} + b_i e^{-i(\Omega_i + \delta_i)t} \right) + H.c. \right]. \quad (\text{S3})$$

For simplicity,  $\tilde{a}$  is now renamed  $a$ . In a first approximation, we consider that the terms oscillating at frequencies close to  $\pm|\Omega_2 - \Omega_1|$  and  $2\Omega_{1,2}$  are filtered out by the optical and mechanical susceptibilities. The removed terms are different in the cases of the isolator and amplifier.

### A. Isolator coupling matrices

Without the fast-rotating terms, the equations of evolution are:

$$\begin{cases} \dot{a} &= i \sum_j (G_{j-} e^{i\Delta t} + G_{j+} e^{-i\Delta t}) b_j - \frac{\kappa}{2} a + \sqrt{\kappa_i} a_{\text{in}}^i + \sqrt{\kappa_e} a_{\text{in}}^e \\ \dot{b}_j &= i\delta_j b_j + i (G_{j-}^* e^{-i\Delta t} + G_{j+}^* e^{i\Delta t}) a - \frac{\gamma_j}{2} b_j + \sqrt{\gamma_j} b_{j,\text{in}} \end{cases} \quad (\text{S4})$$

where  $G_{j\pm} \equiv g_j \alpha_{j\pm}$  are the enhanced optomechanical coupling rates. Here the mechanical damping rates  $\gamma_j$  are the effective damping rates including independent auxiliary optical broadening from their intrinsic damping  $\gamma_j^0$ . The Fourier transform reads:

$$\begin{cases} a(\omega) &= \chi_c(\omega) \left\{ i \sum_j [G_{j-} b_j(\omega + \Delta) + G_{j+} b_j(\omega - \Delta)] + \sqrt{\kappa_i} a_{\text{in}}^i(\omega) + \sqrt{\kappa_e} a_{\text{in}}^e(\omega) \right\} \\ b_j(\omega) &= \chi_{m,j}(\omega) \left\{ i [G_{j-}^* a(\omega - \Delta) + G_{j+}^* a(\omega + \Delta)] + \sqrt{\gamma_j} b_{j,\text{in}}(\omega) \right\} \end{cases} \quad (\text{S5})$$

with electromagnetic and mechanical susceptibilities:

$$\chi_c(\omega) \equiv \frac{1}{\kappa/2 - i\omega}, \quad \chi_{m,j}(\omega) \equiv \frac{1}{\gamma_j/2 - i(\omega + \delta_j)}. \quad (\text{S6})$$

The connection between different frequency components gives rise to a system of Floquet components with a frequency spacing  $\Delta$ . The electromagnetic field components at  $\omega - \Delta$  and  $\omega + \Delta$  that appear in  $b_j(\omega)$  are written:

$$\begin{cases} a(\omega - \Delta) &= \chi_c(\omega - \Delta) \left\{ i \sum_j [G_{j-} b_j(\omega) + G_{j+} b_j(\omega - 2\Delta)] + \sqrt{\kappa_i} a_{\text{in}}^i(\omega - \Delta) + \sqrt{\kappa_e} a_{\text{in}}^e(\omega - \Delta) \right\} \\ a(\omega + \Delta) &= \chi_c(\omega + \Delta) \left\{ i \sum_j [G_{j-} b_j(\omega + 2\Delta) + G_{j+} b_j(\omega)] + \sqrt{\kappa_i} a_{\text{in}}^i(\omega + \Delta) + \sqrt{\kappa_e} a_{\text{in}}^e(\omega + \Delta) \right\}, \end{cases} \quad (\text{S7})$$

However the fields  $b_j(\omega - 2\Delta)$  and  $b_j(\omega + 2\Delta)$  are strongly suppressed by the mechanical susceptibilities for  $\omega \simeq 0$  because  $\gamma_j \sim 1$  kHz remains much smaller than  $\Delta \sim 50$  kHz. Therefore, the system only effectively connects  $b_j(\omega)$  and the first Floquet manifold  $a(\omega - \Delta)$ ,  $a(\omega + \Delta)$ . These two components of the field define the two ports of the device in what follows, which are named respectively 1 and 2 to denote the coupling  $T_{ij}$  and scattering coefficients  $S_{ij}$ . We use the vectors  $A(\omega) \equiv (a(\omega - \Delta) \ a(\omega + \Delta))^T$ ,  $B(\omega) \equiv (b_1(\omega) \ b_2(\omega))^T$ , and similarly defined  $A_{\text{in}}^i(\omega)$ ,  $A_{\text{in}}^e(\omega)$  and  $B_{\text{in}}(\omega)$ . We further introduce the electromagnetic and mechanical susceptibility matrices:

$$\bar{\chi}_c(\omega) \equiv \begin{pmatrix} \chi_c(\omega - \Delta) & \\ & \chi_c(\omega + \Delta) \end{pmatrix}, \quad \bar{\chi}_m(\omega) \equiv \begin{pmatrix} \chi_{m,1}(\omega) & \\ & \chi_{m,2}(\omega) \end{pmatrix} \quad (\text{S8})$$

and the mechanical decoherence rates' square-root matrix  $\sqrt{\gamma} \equiv \text{diag} \{ \sqrt{\gamma_1}, \sqrt{\gamma_2} \}$ . One can write the following matrix equations that assume the form of standard coupled equations with only one phonon field  $B$  and one photon field  $A$ :

$$\begin{cases} A(\omega) &= \bar{\chi}_c(\omega) [\mathcal{G}B(\omega) + \sqrt{\kappa_i} A_{\text{in}}^i(\omega) + \sqrt{\kappa_e} A_{\text{in}}^e(\omega)] \\ B(\omega) &= \bar{\chi}_m(\omega) [\mathcal{H}A(\omega) + \sqrt{\gamma} B_{\text{in}}(\omega)] \end{cases} \quad (\text{S9})$$

with the coupling matrices:

$$\mathcal{G} = i \begin{pmatrix} G_{1-} & G_{2-} \\ G_{1+} & G_{2+} \end{pmatrix} \quad \mathcal{H} = i \begin{pmatrix} G_{1-}^* & G_{1+}^* \\ G_{2-}^* & G_{2+}^* \end{pmatrix}. \quad (\text{S10})$$

### B. Directional amplifier coupling matrices

In the case of the directional amplifier, the mechanical filtering selects different terms of the evolution equations than for the isolator:

$$\begin{cases} \dot{a} &= i \sum_j (G_{j-} e^{i\Delta t} b_j + G_{j+} e^{-i\Delta t} b_j^\dagger) - \frac{\kappa}{2} a + \sqrt{\kappa_i} a_{\text{in}}^i + \sqrt{\kappa_e} a_{\text{in}}^e \\ \dot{b}_j &= i\delta_j b_j + i (G_{j-}^* e^{-i\Delta t} a + G_{j+} e^{-i\Delta t} a^\dagger) - \frac{\gamma_j}{2} b_j + \sqrt{\gamma_j} b_{j,\text{in}} \end{cases} \quad (\text{S11})$$

which gives in Fourier transform:

$$\begin{cases} a(\omega) = \chi_c(\omega) \left\{ i \sum_j \left[ G_{j-} b_j(\omega + \Delta) + G_{j+} b_j^\dagger(\omega - \Delta) \right] + \sqrt{\kappa_i} a_{\text{in}}^i(\omega) + \sqrt{\kappa_e} a_{\text{in}}^e(\omega) \right\} \\ b_j(\omega) = \chi_{m,j}(\omega) \left\{ i \left[ G_{j-}^* a(\omega - \Delta) + G_{j+} a^\dagger(\omega - \Delta) \right] + \sqrt{\gamma_j} b_{j,\text{in}}(\omega) \right\} \end{cases} \quad (\text{S12})$$

With the same approximations as for the isolator, one can show that only  $b_j(\omega)$ ,  $a(\omega - \Delta)$  and  $a^\dagger(\omega + \Delta)$  are coupled (and similarly their hermitian conjugates are coupled). Note that  $a(-\Delta)$  describes fields oscillating at  $\omega_c - \Delta$  while  $a^\dagger(-\Delta)$  describes fields oscillating at  $\omega_c + \Delta$ , from the other port. Changing the definitions of vectors into  $A(\omega) \equiv (a(\omega - \Delta) \ a^\dagger(\omega - \Delta))^T$ , similarly for  $A_{\text{in}}^i(\omega)$ ,  $A_{\text{in}}^e(\omega)$ , and redefining the adequate electromagnetic susceptibility matrix for the amplifier:

$$\bar{\chi}_c(\omega) \equiv \begin{pmatrix} \chi_c(\omega - \Delta) & \\ & \chi_c^*(\omega - \Delta) \end{pmatrix}, \quad (\text{S13})$$

one obtains the same matrix equation as for the isolator S9, but with coupling matrices:

$$\mathcal{G} = i \begin{pmatrix} G_{1-} & G_{2-} \\ -G_{1+}^* & -G_{2+}^* \end{pmatrix} \quad \mathcal{H} = i \begin{pmatrix} G_{1-}^* & G_{1+} \\ G_{2-}^* & G_{2+} \end{pmatrix}. \quad (\text{S14})$$

Note that, as long as the cavity susceptibility is centered on  $\omega = 0$ ,  $\chi_c^*(\omega) = (\chi_c(-\omega))^* = \chi_c(\omega)$ .

### C. Global optical susceptibility and generic scattering matrix

Since equations S9 are valid both for the isolator and the directional amplifier with their own conventions, the development that follows is the same. One can replace the phononic field  $B(\omega)$  expression in the photonic field's  $A(\omega)$ :

$$A = \bar{\chi}_c \left( \mathcal{G} \bar{\chi}_m \mathcal{H} A + \mathcal{G} \bar{\chi}_m \sqrt{\gamma} B_{\text{in}} + \sqrt{\kappa_i} A_{\text{in}}^i + \sqrt{\kappa_e} A_{\text{in}}^e \right) \quad (\text{S15})$$

where frequency dependencies were omitted. The cavity susceptibility is therefore modified into the global susceptibility matrix  $\chi$  defined in the main text by the coupling configuration as  $\chi^{-1} = \bar{\chi}_c^{-1} - \mathcal{G} \bar{\chi}_m \mathcal{H}$  where we identify the matrix  $T$  of the coupling between cavity field components as  $T \equiv -\mathcal{G} \bar{\chi}_m \mathcal{H}$ , and the scattering matrix  $S$  can be computed as indicated in the main text.

## III. ISOLATOR SCATTERING PARAMETERS

The coupling coefficients in the isolator case are

$$\begin{cases} T_{11}(\omega) = |G_{1-}|^2 & \chi_{m,1}(\omega) + |G_{2-}|^2 & \chi_{m,2}(\omega) \\ T_{12}(\omega) = G_{1-} G_{1+}^* & \chi_{m,1}(\omega) + G_{2-} G_{2+}^* & \chi_{m,2}(\omega) \\ T_{21}(\omega) = G_{1-}^* G_{1+} & \chi_{m,1}(\omega) + G_{2-}^* G_{2+} & \chi_{m,2}(\omega) \\ T_{22}(\omega) = |G_{1+}|^2 & \chi_{m,1}(\omega) + |G_{2+}|^2 & \chi_{m,2}(\omega) \end{cases} \quad (\text{S16})$$

Each of the coupling coefficients consists in two terms, which translates the coexistence of the two mechanically-mediated coupling mechanisms between cavity field components. A nonreciprocal coupling situation is furthermore obtained for example when  $T_{12}$  and  $T_{21}$  have different moduli. As previously noted [1], this is only possible because the mechanical susceptibilities are pumped out of resonance, adding a non-zero phase to the transmission paths. This allows susceptibilities  $\chi_{m,j}$  not to be even functions of  $\omega$ . As can be seen from the previous equations S16, this non-parity condition is the condition for  $T_{12}$  and  $T_{21}$  not to be mutual complex conjugates with the same modulus. Enhanced couplings are denoted in terms of cooperativities:

$$G_{1-} = \frac{\sqrt{C_{1-} \kappa \gamma_1}}{2} e^{i\varphi/2}, \quad G_{2-} = \frac{\sqrt{C_{2-} \kappa \gamma_2}}{2} e^{-i\varphi/2}, \quad G_{1+} = \frac{\sqrt{C_{1+} \kappa \gamma_2}}{2}, \quad G_{2+} = \frac{\sqrt{C_{2+} \kappa \gamma_1}}{2}. \quad (\text{S17})$$

This parametrization distributes the only phase degree of freedom  $\varphi = (\theta_{1-} - \theta_{1+}) - (\theta_{2-} - \theta_{2+})$ , where  $\theta_{j\pm}$  is the complex phase of  $G_{j\pm}$ , over the two tones detuned by  $-\Delta$ . The scattering parameters are then:

$$\begin{cases} S_{11}(\omega) = 1 - \kappa_e \chi_c(\omega - \Delta) \frac{1 + \chi_c(\omega + \Delta)T_{22}}{D} \\ S_{12}(\omega) = - \kappa_e \chi_c(\omega - \Delta) \frac{\chi_c(\omega + \Delta)T_{12}}{D} \\ S_{21}(\omega) = - \kappa_e \chi_c(\omega + \Delta) \frac{\chi_c(\omega - \Delta)T_{21}}{D} \\ S_{22}(\omega) = 1 - \kappa_e \chi_c(\omega + \Delta) \frac{1 + \chi_c(\omega - \Delta)T_{11}}{D} \end{cases} \quad (\text{S18})$$

where for simplicity we omitted the  $\omega$  dependence of  $T_{ij}$  and of the common denominator  $D$  which is the determinant of the modified susceptibility matrix  $D(\omega) = (1 + \chi_c(\omega - \Delta)T_{11})(1 + \chi_c(\omega + \Delta)T_{22}) - \chi_c(\omega - \Delta)\chi_c(\omega + \Delta)T_{12}T_{21}$ . These scattering coefficients are represented on Fig. S1.

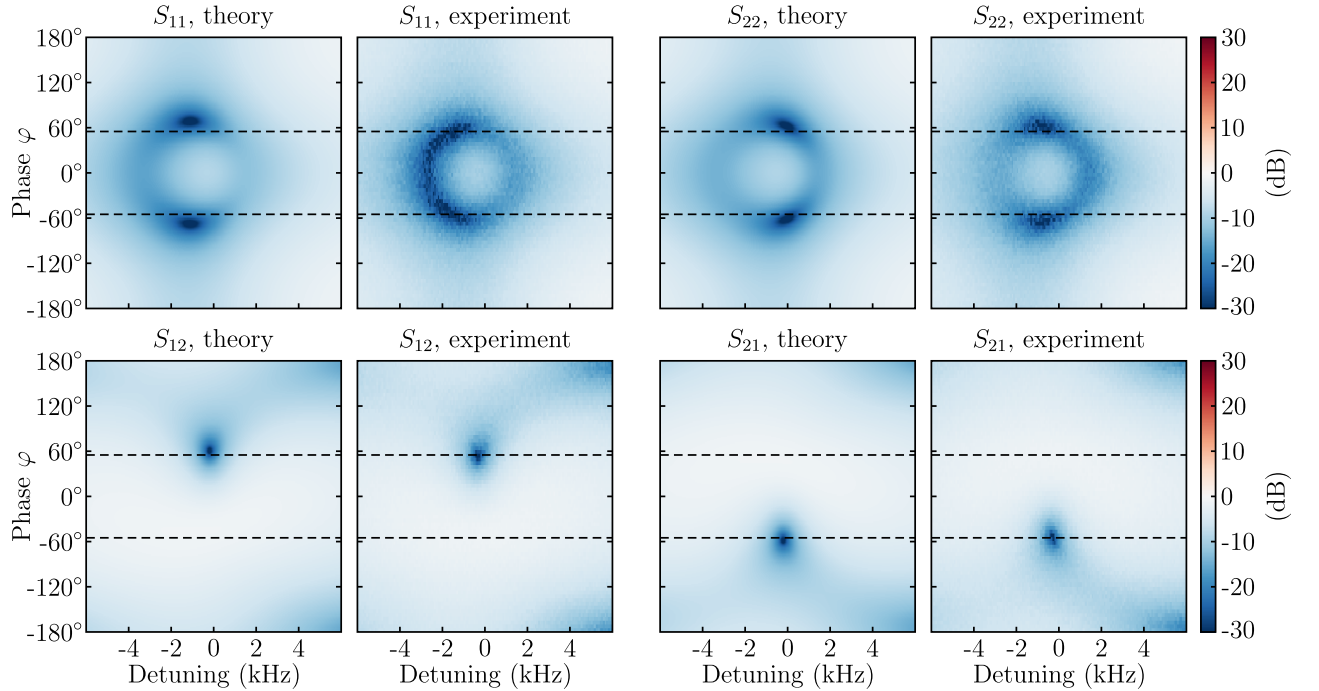

FIG. S1. Measured isolator S-parameters for all phases. The dashed lines indicate optimal directionality phases  $\varphi = \pm 55^\circ$ .

### A. Isolation condition for the isolator

Isolation of port 1 at resonance is obtained if  $|S_{12}(0)| = 0$ , that is if  $|T_{12}(0)| = 0$ , that is:

$$e^{i\varphi} = -\frac{C_{2-}C_{2+}}{C_{1-}C_{1+}} \frac{1 - 2i\delta_1/\gamma_1}{1 - 2i\delta_2/\gamma_2} \quad (\text{S19})$$

For simplicity, let us introduce a dimensionless parameter  $\delta$  and assume that  $\delta_1 = \delta\gamma_1$  and  $\delta_2 = -\delta\gamma_2$ . The requirement on the modulus of S19 becomes a balance condition between cooperativities driving mechanical oscillator 1 and mechanical oscillator 2:

$$C_{1-}C_{1+} = C_{2-}C_{2+}. \quad (\text{S20})$$

If, on the other hand, the detunings  $\delta_1$  and  $\delta_2$  do not compensate exactly for the imbalance between  $\gamma_1$  and  $\gamma_2$  (which is most often the case experimentally), cooperativities may be tuned to recover a modulus of 1 for the right-hand-side

of equation S19. The complex argument of equation S19 furthermore gives the isolation phase:

$$\varphi = \arg \left( \frac{-1 + 2i\delta_1/\gamma_1}{1 - 2i\delta_2/\gamma_2} \right) = \arg \left( \frac{-1 + 2i\delta}{1 + 2i\delta} \right), \quad (\text{S21})$$

which can therefore be tuned as well to recover perfect isolation if by accident  $\delta_1$  and  $\delta_2$  are not proportional to  $\gamma_1$  and  $\gamma_2$ . Isolation of port 2 is obtained for the opposite phase. Note that these conditions are identical to those of isolators and amplifiers using separate cavity modes [1–5], in particular there is no change in the phase requirement due to the off-resonant driving of the system.

### B. Isolator impedance matching

If port 1 is isolated then it features the input port of the device and impedance-matching corresponds to  $|S_{11}(0)| = 0$ , that is:

$$T_{11}(0) = \kappa_e - \frac{1}{\chi_c(-\Delta)} = \frac{\kappa_e - \kappa_i}{2} - i\Delta. \quad (\text{S22})$$

This complex coupling cannot be obtained with identical cooperativities  $C_{1-}$  and  $C_{1+}$ : contrary to previous implementations, impedance-matching now relies on a carefully prepared imbalance of cooperativities depending on detunings  $\delta$  and  $\Delta$ :

$$\begin{cases} C_{1-} = (1 + 4\delta^2) \left( \frac{\kappa_e - \kappa_i - \Delta/\delta}{2\kappa} \right) \\ C_{2-} = (1 + 4\delta^2) \left( \frac{\kappa_e - \kappa_i + \Delta/\delta}{2\kappa} \right) \end{cases} \quad (\text{S23})$$

To satisfy the isolation condition S20, cooperativities  $C_{1+}$  and  $C_{2+}$  have to be  $C_{1+} = \alpha C_{2-}$  and  $C_{2+} = \alpha C_{1-}$  with  $\alpha$  a real, positive coefficient. The value  $\alpha = 1$  ensures simultaneous impedance-matching of port 2. Backward-propagating signals are then neither transmitted nor reflected by the device but fully dissipated. The impedance-matching condition on detuning  $\delta$  is written:

$$\delta = \frac{1}{2} \sqrt{\frac{\kappa(C_{1-} + C_{2-})}{\kappa_e - \kappa_i}} - 1, \quad (\text{S24})$$

which is only possible for sufficient cooperativities.

## IV. DIRECTIONAL AMPLIFIER SCATTERING COEFFICIENTS

Following the same definitions as for the isolator, the directional-amplifier coupling matrix's elements  $T_{ij}$  and scattering coefficients  $S_{ij}$  are

$$\begin{cases} T_{11}(\omega) = |G_{1-}|^2 & \chi_{m,1}(\omega) + |G_{2-}|^2 & \chi_{m,2}(\omega) \\ T_{12}(\omega) = G_{1-}G_{1+} & \chi_{m,1}(\omega) + G_{2-}G_{2+} & \chi_{m,2}(\omega) \\ T_{21}(\omega) = -G_{1-}^*G_{1+}^* & \chi_{m,1}(\omega) - G_{2-}^*G_{2+}^* & \chi_{m,2}(\omega) \\ T_{22}(\omega) = -|G_{1+}|^2 & \chi_{m,1}(\omega) - |G_{2+}|^2 & \chi_{m,2}(\omega) \end{cases}, \quad \begin{cases} S_{11}(\omega) = 1 - \kappa_e \chi_c(\omega - \Delta) \frac{1 + \chi_c^*(\omega - \Delta)T_{22}}{D} \\ S_{12}(\omega) = -\kappa_e \chi_c(\omega - \Delta) \frac{\chi_c^*(\omega - \Delta)T_{12}}{D} \\ S_{21}(\omega) = -\kappa_e \chi_c^*(\omega - \Delta) \frac{\chi_c(\omega - \Delta)T_{21}}{D} \\ S_{22}(\omega) = 1 - \kappa_e \chi_c^*(\omega - \Delta) \frac{1 + \chi_c(\omega - \Delta)T_{11}}{D} \end{cases} \quad (\text{S25})$$

with the denominator  $D(\omega) = (1 + \chi_c(\omega - \Delta)T_{11})(1 + \chi_c^*(\omega - \Delta)T_{22}) - \chi_c(\omega - \Delta)\chi_c^*(\omega - \Delta)T_{12}T_{21}$ . Note that the only phase degree of freedom of the amplifier is  $\varphi = (\theta_{1-} + \theta_{1+}) - (\theta_{2-} + \theta_{2+})$  where  $\theta_{j\pm}$  is the complex phase of  $G_{j\pm}$ , unlike the isolator's which is  $(\theta_{1-} - \theta_{1+}) - (\theta_{2-} - \theta_{2+})$ . However, the parametrization S17 of enhanced couplings  $G_{j\pm}$  used for the isolator distributes this phase over the two tones detuned by  $-\Delta$  and it can be employed as well in the case of the amplifier. These scattering coefficients are represented on Fig. S2.

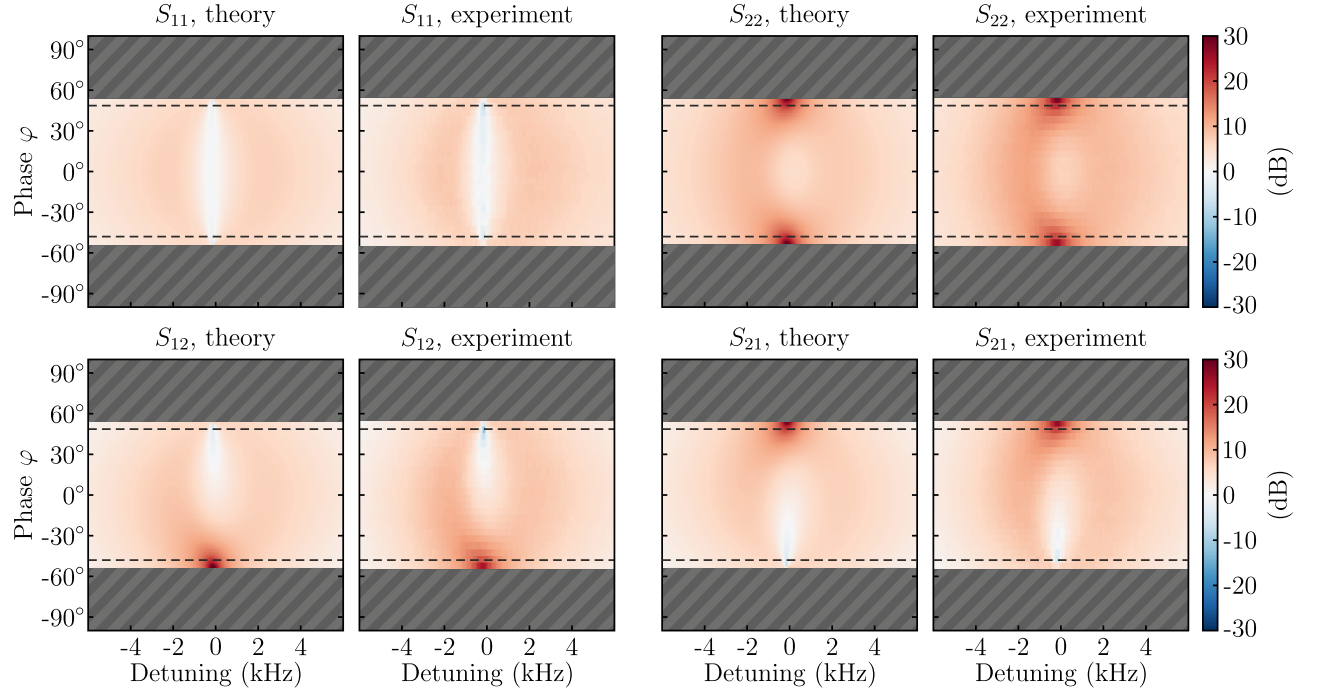

FIG. S2. Measured amplifier S-parameters for all phases. On experimental data plots, the gray dashed region indicates the region where the device is unstable  $|\varphi| > \pm 55^\circ$ . On theoretical plots, the gray dashed region indicates phases for which one of the system's eigenvalue has a negative real-part. A good agreement is found not only between theoretical and measured scattering parameters, but also on the position of the instability thresholds. The dashed lines indicate optimal directionality phases  $\varphi = \pm 48^\circ$ .

### A. Amplifier isolation and impedance matching conditions

The isolation condition and impedance matching condition of port 1 are exactly the same for the amplifier as for the isolator. Namely, if  $\delta_1 = \delta\gamma_{1,\text{eff}}$  and  $\delta_2 = -\delta\gamma_{2,\text{eff}}$ :  $C_{1-}C_{1+} = C_{2-}C_{2+}$  and  $\varphi = \arg\left(\frac{-1+2i\delta}{1+2i\delta}\right)$  are required for isolation and condition S23 for impedance matching. As in the case of the isolator, to maintain both isolation and impedance matching of port 1, cooperativities  $C_{j+}$  should be  $C_{1+} = \alpha C_{2-}$  and  $C_{2+} = \alpha C_{1-}$ . However, unlike the case of the isolator, there is no value of  $\alpha$  which can grant impedance-matching of port 2 simultaneously. Signals injected on port 2, that are not transmitted port 1 since it is isolated, are back-scattered with some gain rather than dissipated as in the isolator, which translates as a high  $|S_{22}|^2$  reflectivity.

### B. Gain

We again assume that port 1 is isolated ( $T_{12}(0) = 0$ ) and impedance-matched. Taking furthermore the limit of ideal cavities  $\kappa_i/\kappa \ll 1$  and high cooperativity  $C_- \gg 1$ , the forward gain is

$$|S_{21}(0)|^2 = \frac{4C_{1-}C_{1+}}{(C_{1-} + C_{2-})^2 \frac{\Delta^2}{\kappa^2} + \left(\frac{C_{1-} + C_{2-}}{2} - C_{1+}\right)^2}. \quad (\text{S26})$$

In the limit of small detunings  $\Delta/\kappa \ll 1$ , impedance-matching is achieved for equal red-sideband cooperativities  $C_{1-} = C_{2-} = C_-$  and blue-sideband-cooperativities  $C_{1+} = C_{2+} = C_+$ . The gain in this limit is similar to the one found for 2-cavity-modes systems [1, 5]

$$|S_{21}(0)|^2 = \frac{4C_-C_+}{(C_- - C_+)^2}. \quad (\text{S27})$$

Therefore, while the theoretical gain S27 is unlimited in the 2-cavity-modes case S27 as  $C_+$  can be brought arbitrarily close to  $C_-$  to cancel out the denominator, there exists a trade-off cooperativity in the 2-Floquet-mode case S26 presented in this work associated with an upper bound on the gain.

## V. EXPERIMENTAL METHODS

### A. Measurement

The measurement of the frequency-converting response is done by sending a probe tone together with the pumps. Its frequency is swept across the processes' resonance around  $\omega_c - \Delta$  and  $\omega_c + \Delta$ , and the spectrum of the cavity output is measured for each probe frequency (see Fig. S3 such a spectrum in gray solid line). These spectra consist of a background of noise and two peaks: one at the frequency of the probe because of reflection on the device, and one one at the frequency to which the device converts. The former allows to characterize  $S_{11}$  or  $S_{22}$ , and the latter  $S_{12}$  or  $S_{21}$ , depending on which port is driven. The amplitude of these peaks, initially measured from the bottom of the cavity response, is finally corrected by the depth of the cavity response to get the net gains of the device.

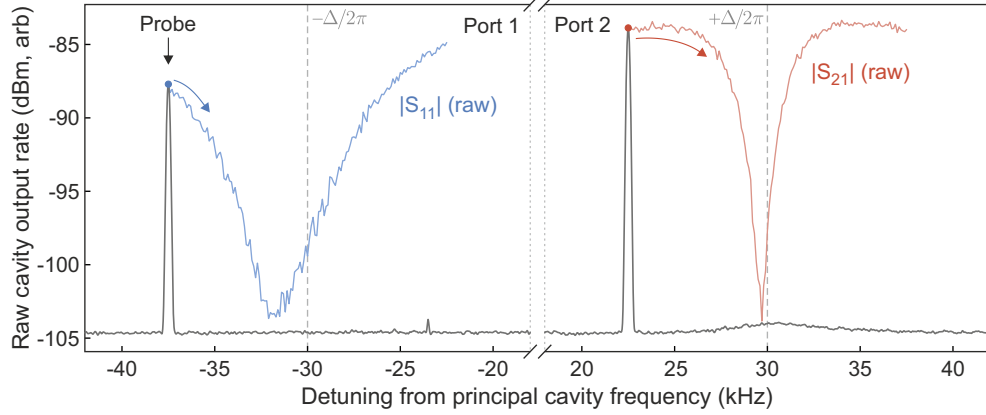

FIG. S3. Raw spectrum measurement (gray line) of the isolator principal cavity's output rate on the two frequency ranges around  $\pm\Delta$ , while probing port 1 with a frequency indicated with a black arrow. The peak on the left corresponds to reflection of this probe on port 1 while the peak on the right corresponds to frequency-conversion to port 2. Measuring these two peaks amplitudes, represented as a blue and a red dot respectively, while scanning the probe frequency in port 1 allows to record raw versions of  $S_{11}$  (light blue line) and  $S_{21}$  (light red line). Port 2 is then probed in the same way to record  $S_{22}$  and  $S_{21}$ . One can clearly see the bump in noise amplitude at port 2's frequency, which is here the isolated port and therefore displays more noise than port 1 (see main text.)

### B. Noise calibration

The spectra measured for each probe frequency, less the two peaks at the probe frequency and the converted frequency, are averaged together and the result is calibrated to reflect the photonic noise on each of the device's ports. This calibration is based on the knowledge of the background noise coming mainly from a cryogenic amplifier (HEMT) used in the measurement line, following the Y-factor method. During the calibration stage, a noise of known amplitude emitted by a  $R = 50\Omega$  resistor is measured with the same detection line as the amplifier (see Figure S4). The measured voltage noise is then a sum of contributions from the resistor and from the HEMT amplifier:  $S_V(\omega) = G_H R \hbar \omega \left[ \frac{1}{2} \coth \left( \frac{\hbar \omega}{2 k_B T} \right) + n_H(\omega) \right]$ , where  $G_H$  is a dimensionless gain of the measurement line and  $n_H$  the added number of photons from the HEMT. Sweeping the temperature of the resistor allows to fit both of these values to  $10 \log_{10} G_H = 69 \text{ dB}$  and  $n_H = 11.4$  quanta at the frequency of the cavity. During the experiment, the spectrum of the background noise  $S_H$  from the HEMT is again measured and compared to the measured cavity output spectrum at port  $j$ :  $S_{j,\text{mes}} = S_{j,\text{out}} + S_H$ . The noise from port  $j$  of the device is:

$$n_{j,\text{out}}(\omega) = n_H(\omega) \left( \frac{S_{j,\text{mes}}(\omega)}{S_H(\omega)} - 1 \right). \quad (\text{S28})$$

Finally, stray power from each of the six pumps used to drive the system in each experiment is cancelled before reaching the HEMT to avoid its saturation so that its behavior remains the same as in the calibration stage.

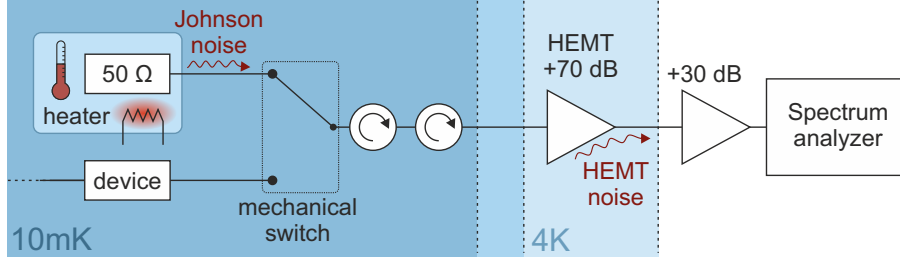

FIG. S4. Background noise calibration simplified setup schematic.

### C. Analysis

The data is fitted with the expressions of the isolator and amplifier parameters from the text. A small mechanical frequency modification calibrated together with the amount of auxiliary cooling is taken into account as a modification of the pump detunings  $\delta_j$ . A small modification of the principal cavity frequency of 110 kHz is also taken into account.

## VI. AUXILIARY COOLING

The auxiliary cavity is driven by two tones of frequencies  $\omega_c^a - \Delta^a - \Omega_1$  and  $\omega_c^a + \Delta^a - \Omega_2$  with  $\omega_c^a$  the angular frequency of the auxiliary cavity mode and  $\Delta^a = -50$  kHz a detuning larger than the final effective mechanical linewidths to avoid additional coupling between mechanical modes. Driving the two sidebands at the same time, the following cooling parameters are achieved:

| Isolator                          | Mode 1      | Mode 2      |
|-----------------------------------|-------------|-------------|
| Effective phonon occupancy $n_j$  | 4.0 phonons | 8.9 phonons |
| Effective damping rate $\gamma_j$ | 1.739 kHz   | 1.876 Hz    |
| Amplifier                         | Mode 1      | Mode 2      |
| Effective phonon occupancy $n_j$  | 2.9 phonons | 8.1 phonons |
| Effective damping rate $\gamma_j$ | 1.567 kHz   | 898 Hz      |

Numbers of quanta are given here without the vacuum fluctuations contribution. A small frequency modification of each mode is observed due to the combined optical spring effects of both pumps on each mode. This frequency change is taken into account into the analysis of the isolator's and amplifier's results. The pump detunings  $\delta_j$  announced in the text  $\delta_1/2\pi = -\delta_2/2\pi = 1000$  Hz are given from the natural frequencies and do not include this frequency modification.

## VII. CROSS-COUPLING TERMS

In this section we derive the devices S-parameters and noise figure expressions if we take into account cavity field components oscillating at  $\pm\Delta_{21}$  that were neglected in the basic theory section. These terms arise because each pump intended to drive one mechanical mode's sideband drives the other in a certain proportion due to their frequency proximity. We introduce the angular mechanical frequency difference  $\{\Delta_{\bar{j}j} = \Omega_{\bar{j}} - \Omega_j\}_{j=1,2}$  where  $\bar{j}$  is "not  $j$ ", that is,  $\bar{j} = 2$  if  $j = 1$  and  $\bar{j} = 1$  if  $j = 2$ . We also introduce cross-coupling amplitudes:  $J_{j\pm} = g_j \alpha_{\bar{j}\pm}$ , that is, the parasitic coupling of mode  $j$  to a pump intended to drive the other mode  $\bar{j}$ .

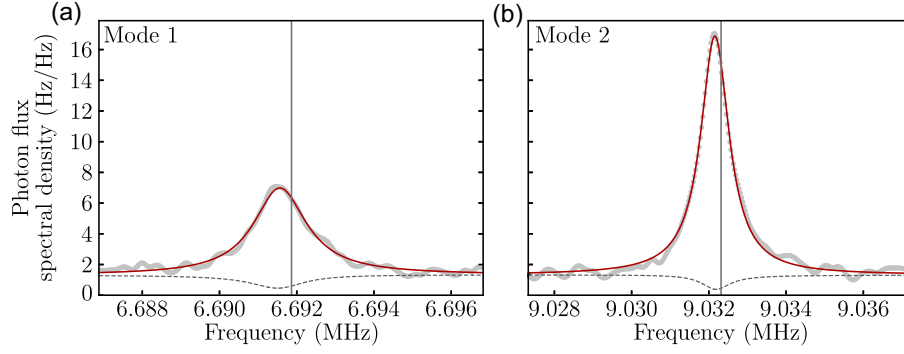

FIG. S5. Mechanical modes auxiliary cooling calibration. **a.** Spectrum of the auxiliary cavity output at the frequency  $(\omega_c^a - \Delta^a)/2\pi$  displaying the signature of mode 1's mechanical spectrum. **b.** Same measurement at frequency  $(\omega_c^a + \Delta^a)/2\pi$  displaying the signature of mode 2's mechanical spectrum. Gray dots: measurement, red solid line: fit, dashed dark gray line: contribution of the cavity occupancy to the spectrum, vertical line: bare frequency of either mode.

### A. Isolator case

The perturbed equations of motion are written:

$$\begin{cases} \dot{a} = i \sum_j \left( G_{j-} e^{i\Delta t} + G_{j+} e^{-i\Delta t} + J_{j-} e^{i(\Delta + \Delta_{jj})t} + J_{j+} e^{-i(\Delta - \Delta_{jj})t} \right) b_j - \frac{\kappa}{2} a + \sqrt{\kappa_i} a_{\text{in}}^i + \sqrt{\kappa_e} a_{\text{in}}^e \\ \dot{b}_j = i\delta_j b_j + i \left( G_{j-}^* e^{-i\Delta t} + G_{j+}^* e^{i\Delta t} + J_{j-}^* e^{-i(\Delta + \Delta_{jj})t} + J_{j+}^* e^{i(\Delta - \Delta_{jj})t} \right) a - \frac{\gamma_j}{2} b_j + \sqrt{\gamma_j} a_{j\text{in}} \end{cases} \quad (\text{S29})$$

We introduce the “cross-coupling” matrices

$$\mathcal{G}^+ = i \begin{pmatrix} J_{1-} & 0 \\ J_{1+} & 0 \end{pmatrix}, \quad \mathcal{G}^- = i \begin{pmatrix} 0 & J_{2-} \\ 0 & J_{2+} \end{pmatrix}, \quad \mathcal{H}^+ = i \begin{pmatrix} 0 & 0 \\ J_{2-}^* & J_{2+}^* \end{pmatrix}, \quad \mathcal{H}^- = i \begin{pmatrix} J_{1-}^* & J_{1+}^* \\ 0 & 0 \end{pmatrix}. \quad (\text{S30})$$

Furthermore, for each frequency-dependent matrix  $F(\omega)$ , we denote  $F^{(n)} = F(\omega + n\Delta_{21})$  the  $n$ -th Floquet manifold. The equations can be written again under a matrix form similar to equation S9:

$$\begin{cases} A^{(n)} = \bar{\chi}_c^{(n)} \left[ \mathcal{G} B^{(n)} + \mathcal{G}^- B^{(n-1)} + \mathcal{G}^+ B^{(n+1)} + \sqrt{\kappa} A_{\text{in}}^{(n)} \right] \\ B^{(n)} = \bar{\chi}_m^{(n)} \left[ \mathcal{H} A^{(n)} + \mathcal{H}^- A^{(n-1)} + \mathcal{H}^+ A^{(n+1)} + \sqrt{\gamma} B_{\text{in}}^{(n)} \right] \end{cases} \quad (\text{S31})$$

Notice that the terms  $\sqrt{\kappa_i} A_{\text{in}}^i + \sqrt{\kappa_e} A_{\text{in}}^e$  were condensed into the notation  $\sqrt{\kappa} A_{\text{in}}^{(n)}$  for simplicity in this section. The replacement of  $A^{(n)}$  and  $A^{(n\pm 1)}$  in the second equation gives a relationship between  $B^{(n)}$ ,  $B^{(n\pm 1)}$ ,  $B^{(n\pm 2)}$  and noise terms  $B_{\text{in}}^{(n)}$ ,  $A_{\text{in}}^{(n)}$  and  $A_{\text{in}}^{(n\pm 1)}$ . However, the elements of  $\bar{\chi}_m^{(n)} = \bar{\chi}_m(\omega + n\Delta_{21})$  are negligibly small for  $n \neq 0$ . Therefore, any term containing these matrices can be removed and this relation is written for  $n = 0$ :

$$\begin{aligned} B^{(0)} = \bar{\chi}_m^{(0)} \Big[ & \mathcal{H} \bar{\chi}_c^{(0)} \mathcal{G} B^{(0)} + \mathcal{H} \bar{\chi}_c^{(0)} \sqrt{\kappa} A_{\text{in}}^{(0)} + \sqrt{\gamma} B_{\text{in}}^{(0)} \\ & + \left( \mathcal{H}^- \bar{\chi}_c^{(-1)} \mathcal{G}^+ + \mathcal{H}^+ \bar{\chi}_c^{(1)} \mathcal{G}^- \right) B^{(0)} + \mathcal{H}^- \bar{\chi}_c^{(-1)} \sqrt{\kappa} A_{\text{in}}^{(-1)} + \mathcal{H}^+ \bar{\chi}_c^{(1)} \sqrt{\kappa} A_{\text{in}}^{(1)} \Big]. \end{aligned} \quad (\text{S32})$$

The terms of the first line are the ones obtained in the strictest approximation used in the beginning, while the terms of the second line come from the relaxing of this approximation. We can see that the perturbation corresponds to adding back-action terms to the mechanical susceptibilities:

$$\bar{\chi}_m^{-1}(\omega) \rightarrow \bar{\chi}_m^{-1'}(\omega) = \bar{\chi}_m^{-1}(\omega) - [\mathcal{H}^- \bar{\chi}_c(\omega - \Delta_{21}) \mathcal{G}^+ + \mathcal{H}^+ \bar{\chi}_c(\omega + \Delta_{21}) \mathcal{G}^-] \quad (\text{S33})$$

and additional noise terms from off-resonant cavity field components that impact the resonant component  $A^0 = A(\omega)$  as:

$$A(\omega) = \bar{\chi}_c(\omega) \left[ \dots + \mathcal{G} \bar{\chi}_m'(\omega) \mathcal{H}^- \bar{\chi}_c(\omega - \Delta_{21}) \sqrt{\kappa} A_{\text{in}}(\omega - \Delta_{21}) + \mathcal{G} \bar{\chi}_m'(\omega) \mathcal{H}^+ \bar{\chi}_c(\omega + \Delta_{21}) \sqrt{\kappa} A_{\text{in}}(\omega + \Delta_{21}) \right]. \quad (\text{S34})$$

With the coupling matrices found for the isolator case, the modified mechanical susceptibilities of each modes are:

$$\begin{cases} \chi'_{m,1}(\omega) = \chi_{m,1}^{-1}(\omega) + |J_{1-}|^2 \chi_c(\omega - \Delta - \Delta_{21}) + |J_{1+}|^2 \chi_c(\omega + \Delta - \Delta_{21}) \\ \chi'_{m,2}(\omega) = \chi_{m,2}^{-1}(\omega) + |J_{2-}|^2 \chi_c(\omega - \Delta + \Delta_{21}) + |J_{2+}|^2 \chi_c(\omega + \Delta + \Delta_{21}) \end{cases} \quad (\text{S35})$$

The effect on each mechanical oscillator is dynamical backaction from each of the two pumps driving the other oscillator, which mainly amounts to optical damping in the case of the isolator. This parasitic effect furthers mechanical oscillators' active cooling down to  $n_{1\text{eff}} = 3$  and  $n_{2\text{eff}} = 6$  phonons, resulting in even lower isolator added noise on both ports, and increases the bandwidth of the isolation (3 kHz when the mechanical linewidth modified only by controlled auxiliary cooling is around 1 kHz for each mode) as has been previously noted [4].

### B. Directional amplifier case

The perturbed equations of motion for the directional amplifier are:

$$\begin{cases} \dot{a} = i \sum_j \left[ (G_{j-} e^{i\Delta t} + J_{j-} e^{i(\Delta + \Delta_{jj})t}) b_j + (G_{j+} e^{-i\Delta t} + J_{j+} e^{-i(\Delta + \Delta_{jj})t}) b_j^\dagger \right] - \frac{\kappa}{2} a + \sqrt{\kappa_i} a_{\text{in}}^i + \sqrt{\kappa_e} a_{\text{in}}^e \\ \dot{b}_j = i \delta_j b_j + i \left[ (G_{j-}^* e^{-i\Delta t} + J_{j-}^* e^{-i(\Delta + \Delta_{jj})t}) a + (G_{j+} e^{-i\Delta t} + J_{j+} e^{-i(\Delta + \Delta_{jj})t}) a^\dagger \right] - \frac{\gamma_j}{2} b_j + \sqrt{\gamma_j} b_{j,\text{in}}. \end{cases} \quad (\text{S36})$$

Defining the corresponding cross-coupling matrices

$$\mathcal{G}^+ = i \begin{pmatrix} J_{1-} & 0 \\ -J_{1+}^* & 0 \end{pmatrix}, \quad \mathcal{G}^- = i \begin{pmatrix} 0 & J_{2-} \\ 0 & -J_{2+}^* \end{pmatrix}, \quad \mathcal{H}^+ = i \begin{pmatrix} 0 & 0 \\ J_{2-}^* & J_{2+} \end{pmatrix}, \quad \mathcal{H}^- = i \begin{pmatrix} J_{1-}^* & J_{1+} \\ 0 & 0 \end{pmatrix}, \quad (\text{S37})$$

one gets exactly the same perturbed equations as for the isolator S31. Therefore, equations S31-S34 stand in the directional amplifier case as well. The effect of cross-coupling again amounts to a modification of the mechanical susceptibility and additional off-resonant electromagnetic noise. Using the coupling matrices of the amplifier, one can write the modified susceptibility as

$$\begin{cases} \chi'_{m,1}(\omega) = \chi_{m,1}^{-1}(\omega) + |J_{1-}|^2 \chi_c(\omega - \Delta - \Delta_{21}) - |J_{1+}|^2 \chi_c^*(\omega - \Delta - \Delta_{21}) \\ \chi'_{m,2}(\omega) = \chi_{m,2}^{-1}(\omega) + |J_{2-}|^2 \chi_c(\omega - \Delta + \Delta_{21}) - |J_{2+}|^2 \chi_c^*(\omega - \Delta + \Delta_{21}). \end{cases} \quad (\text{S38})$$

In this case the dynamical back-action induced by parasitic coupling consists of both damping and anti-damping terms.

## VIII. ANALYSIS OF DEVICES NOISE

The symmetrized output spectra of ports 1 and 2 of the device are:

$$\begin{aligned} S_{\text{out},1}(\omega) &= \frac{1}{4} \int_{-\infty}^{\infty} \frac{d\omega'}{2\pi} \left\langle a_{\text{out}}^\dagger(\omega + \Delta) a_{\text{out}}(\omega' - \Delta) + a_{\text{out}}(\omega - \Delta) a_{\text{out}}^\dagger(\omega' + \Delta) \right\rangle + [\omega \leftrightarrow \omega'] \\ S_{\text{out},2}(\omega) &= \frac{1}{4} \int_{-\infty}^{\infty} \frac{d\omega'}{2\pi} \left\langle a_{\text{out}}^\dagger(\omega - \Delta) a_{\text{out}}(\omega' + \Delta) + a_{\text{out}}(\omega + \Delta) a_{\text{out}}^\dagger(\omega' - \Delta) \right\rangle + [\omega \leftrightarrow \omega'] \end{aligned} \quad (\text{S39})$$

Noise correlators are:  $\langle a_{\text{in}}^{i\dagger}(\omega) a_{\text{in}}^i(\omega') \rangle = 2\pi n_c^i \delta(\omega + \omega')$  and  $\langle a_{\text{in}}^{i\dagger}(\omega) a_{\text{in}}^i(\omega') \rangle = 2\pi(n_c^i + 1)\delta(\omega + \omega')$  and similar definitions for other noise terms. The total devices' noise is modelled by three types of such operators representing: (1) noise from the mechanical oscillators' thermal and vacuum fluctuations  $b_{j,\text{in}}$ , which cause the major part of the total noise, (2) fluctuations from the cavity's environment  $a_{\text{in}}^i$  and (3) fluctuations from the cavity's input coupler  $a_{\text{in}}^e$ , which are only vacuum fluctuations with adequate filtering of transmission lines. Noise operators from different origins are assumed to be uncorrelated. We will here neglect the additional non-RWA noise terms of equation S34 and consider only contributions from:

$$A(\omega) = [\bar{\chi}_c^{-1}(\omega) - \mathcal{G} \bar{\chi}_m(\omega) \mathcal{H}]^{-1} \left( \mathcal{G} \bar{\chi}_m(\omega) \sqrt{\gamma} B_{\text{in}}(\omega) + \sqrt{\kappa_i} A_{\text{in}}^i(\omega) + \sqrt{\kappa_e} A_{\text{in}}^e(\omega) \right). \quad (\text{S40})$$

The modified optical susceptibility introduced in the main text:

$$\chi(\omega) \equiv (\bar{\chi}_c^{-1}(\omega) + T(\omega))^{-1} \quad (\text{S41})$$

represents a scattering matrix internal to the device that relates intracavity fields to drive terms:  $A = \chi A_{\text{in}}$  in the same way as the scattering matrix relates the output cavity fields to drive terms  $A_{\text{out}} = S A_{\text{in}}$ . Importantly,  $\chi(\omega)$  translates isolation in the same way as  $S(\omega)$  (e.g port 1 is isolated if  $\chi_{12}(0) = 0$ ).

The total output noise at port  $i$  is:

$$S_{\text{out},i}(\omega) = M_{i1} \left( n_{m,1} + \frac{1}{2} \right) + M_{i2} \left( n_{m,2} + \frac{1}{2} \right) + Y_i \left( n_c^i + \frac{1}{2} \right) + Z_i \left( n_c^e + \frac{1}{2} \right) \quad (\text{S42})$$

with coefficients:

$$M_{ij} \equiv \kappa_e \left| (\chi \mathcal{G} \bar{\chi}_m \sqrt{\gamma})_{ij} \right|^2, \quad Y_i \equiv \kappa_e \kappa_i \sum_j |\chi_{ij}|^2, \quad Z_i \equiv \sum_j |S_{ij}|^2. \quad (\text{S43})$$

### A. Supplementary information to Fig. 4 of the main text

We supplement Fig. 4(c) and (d) of the main text showing the measured amplifier noise with theoretical plots using no free parameters, shown on Fig. S6 to show the good agreement of the result derived in the previous section with the measured noise.

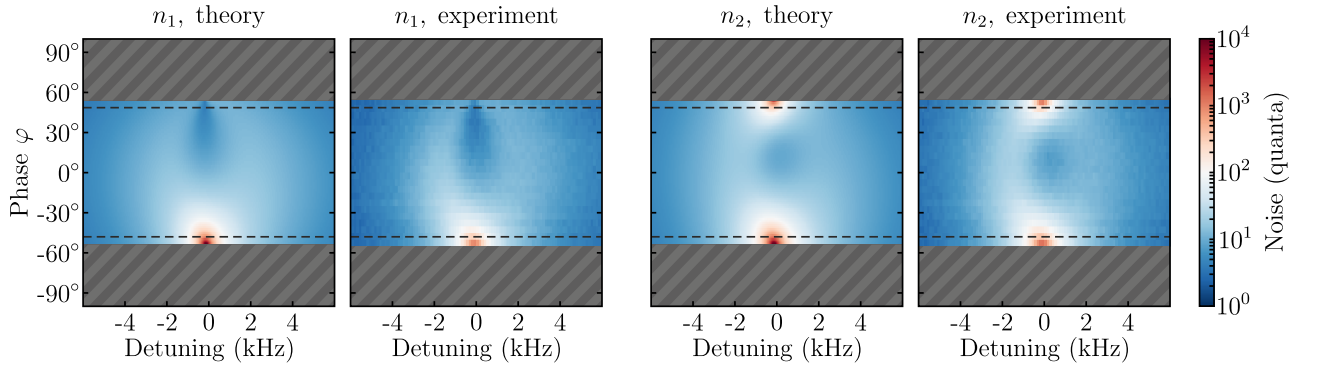

FIG. S6. Measured amplifier noise spectra at both ports for all phases. The gray dashed region indicates the region where the device is unstable  $|\varphi| > \pm 55^\circ$ . The dashed lines indicate optimal directionality phases  $\varphi = \pm 48^\circ$ .

### B. Analysis of paths taken by noise

#### 1. Isolated port

Let us analyze noise at port 1, which is assumed to be isolated, in the case of the isolator. Coefficient  $M_{11}$  writes

$$M_{11}(\omega) = \kappa_e \left| G_{1-} \chi_{11}(\omega) - G_{1+} \chi_{12}(\omega) \right|^2 |\chi_{m,1}(\omega)|^2 \gamma_1 \quad (\text{S44})$$

The first term describes how mechanical noise from oscillator 1 is converted into cavity noise through  $G_{1-}$  (and is modified by the backaction factor  $\chi_{11}$ ). The second term describes how the same noise is converted into fluctuations at the other port's (port 2's) frequency and then propagated back to port 1 through the two paths involved in  $\chi_{12}$ . If port 1 is isolated, these two paths interfere destructively:  $\chi_{12} = 0$  and only the first term remains. If furthermore this port is impedance matched  $\chi_{11} = 1/\kappa_e$ , using condition S23:

$$M_{11}(0) = \frac{\kappa_e - \kappa_i + \Delta/\delta}{2\kappa_e}. \quad (\text{S45})$$

Finally, in the ideal cavity limit  $\kappa_i = 0$  and small detuning approximation  $\Delta \ll \kappa$ , we recover the ideal value [1]  $M_{11}(0) \simeq \frac{1}{2}$ . The same reasoning applies to oscillator 2's noise impact on the isolated port. Cavity noise, on the other hand, propagates exactly as signal in the device, except that internally-originated noise does not undergo external reflection on ports and is scattered by  $\chi$  instead of  $S$ . If port 1 is isolated, cavity noise at port 2's frequency has no contribution on it and the sum in  $Y_1$  and  $Z_1$  are limited to the first term. Furthermore enforcing impedance matching  $\chi_{11}(0) = 1/\kappa_e$ :

$$Y_1(0) = \frac{\kappa_i}{\kappa_e}, \quad Z_1(0) = 0. \quad (\text{S46})$$

## 2. Non-isolated port

Mechanical oscillator 1's contribution to noise at port 2, assumed to be the output port, is written for the isolator:

$$M_{21}(\omega) = \kappa_e \left| G_{1+}\chi_{22}(\omega) - G_{1-}\chi_{21}(\omega) \right|^2 |\chi_{m,1}(\omega)|^2 \gamma_1 \quad (\text{S47})$$

The two terms of  $\chi_{21}$  do not interfere destructively this time, but enforcing isolation and impedance matching brings  $\chi_{21}$  and  $\chi_{22}$  to share the same phase. Therefore, the two terms of Eq. (S47) have a phase difference of  $\pi + \varphi/2$ . At high cooperativities, according to Eq. (S21) and Eq. (S24), the isolation phase  $\varphi$  tends towards zero. Furthermore the two terms tend towards the same amplitude. Therefore this interference is generally partially destructive and tends towards completely destructive at high cooperativities. The forward noise is then only contributed by cavity occupancy which is typically only vacuum fluctuations, making the isolator's forward noise and the amplifier's added noise tend towards the quantum limit of a half photon at high cooperativities.

- 
- [1] D. Malz, L. D. Tóth, N. R. Bernier, A. K. Feofanov, T. J. Kippenberg, and A. Nunnenkamp, "Quantum-Limited Directional Amplifiers with Optomechanics," *Phys. Rev. Lett.* **120**, 023601 (2018).
  - [2] S. Barzanjeh, M. Wulf, M. Peruzzo, M. Kalaei, P. B. Dieterle, O. Painter, and J. M. Fink, "Mechanical on-chip microwave circulator," *Nat. Commun.* **8**, 953 (2017).
  - [3] G. A. Peterson, F. Lecocq, K. Cicak, R. W. Simmonds, J. Aumentado, and J. D. Teufel, "Demonstration of efficient nonreciprocity in a microwave optomechanical circuit," *Phys. Rev. X* **7**, 031001 (2017).
  - [4] N. R. Bernier, L. D. Tóth, A. Koottandavida, M. A. Ioannou, D. Malz, A. Nunnenkamp, A. K. Feofanov, and T. J. Kippenberg, "Nonreciprocal reconfigurable microwave optomechanical circuit," *Nat. Commun.* **8**, 604 (2017).
  - [5] L. Mercier de Lépinay, E. Damskäg, C. F. Ockeloen-Korppi, and M. A. Sillanpää, "Realization of Directional Amplification in a Microwave Optomechanical Device," *Phys. Rev. Applied* **11**, 034027 (2019).
